# Supplementary material for: Finite width of anyons changes their braiding signature
Source: arXiv:2311.15094 source file (2024-07-22)
Supplement: Supplementary file 1 [file supplemental_finite_width_anyons_resub.pdf]

## Supplemental material for
## "Finite width of anyons changes their braiding signature "

K. Iyer,* F. Ronetti, B. Grémaud, T. Martin, J. Rech, and T. Jonckheere
*Aix Marseille Univ, Université de Toulon, CNRS, CPT, Marseille, France*
(Dated: March 12, 2024)

### I. CHIRAL LUTTINGER LIQUID THEORY OF QUANTUM HALL EDGES

In this section, we review the basics of bosonic theory of a general Abelian quantum Hall edge, and we show its application to the case of the filling factor $\nu = 2/5$. The FQHE edges are modeled as chiral Luttinger liquids with a general Abelian quantum Hall edge being described by the action [S1, S2]

$$S = \frac{1}{4\pi}\int dxdt \sum_{i=1}^{N}\left[-\chi_i \partial_x\phi_i\partial_t\phi_i - v_i(\partial_x\phi_i)^2\right] \tag{S1}$$

where $\phi_i$ denote the bosonic modes on the edge, $v_i > 0$ denote the propagation velocity of $i-$th bosonic mode, and $\chi_i = \pm 1$ denote their chiralities, with $i \in \{1, \ldots, N\}$. The bosonic fields satisfy commutation relations given by

$$[\phi_i(x,t), \phi_j(x',t')] = i\pi\delta_{ij}\mathrm{Sign}(X_i - X_j') \tag{S2}$$

where $X_i = -\chi_i x + t$. The charge density $\rho$ and the conserved current $J$ on the edge are given by

$$\begin{aligned} \rho &= \frac{1}{2\pi}\sum_i q_i\partial_x\phi_i \\ J &= -\frac{1}{2\pi}\sum_i q_i\partial_t\phi_i \end{aligned} \tag{S3}$$

where $q_i^2 e^2/h$ is the conductance of the $i$-th bosonic mode, $e$ is the electronic charge, and $h$ the Planck's constant. The conductance is related to the bulk filling fraction $\nu$ of the FQHE liquid via

$$\sum_i \chi_i q_i^2 = \nu \tag{S4}$$

The edge hosts quasiparticle (qp) operators of the form

$$\psi_{\mathbf{g}} \sim e^{i\mathbf{g}\cdot\boldsymbol{\phi}} \tag{S5}$$

where vectors with $N$ components are denoted in bold, and $\mathbf{A}.\mathbf{B} \equiv \sum_i \chi_i A_i B_i$.

The spectrum of quasiparticle operators allowed in a given edge theory can be found in the following manner. First, we find a set of $N$ electron operators $\psi_{\mathbf{e}_\alpha} \sim e^{i\mathbf{e}_\alpha\cdot\boldsymbol{\phi}}$ on the edge by demanding it to satisfy the following relations expected of an electronic excitation

$$\begin{aligned} \{\psi_{\mathbf{e}_\alpha}(x,t), \psi_{\mathbf{e}_\alpha}(x',t)\} &= 0, \\ \psi_{\mathbf{e}_\alpha}(x,t)\psi_{\mathbf{e}_\beta}(x',t) \pm \psi_{\mathbf{e}_\beta}(x',t), \psi_{\mathbf{e}_\alpha}(x,t) &= 0, \\ \left[J^0(x,t), \psi_{\mathbf{e}_\alpha}(x',t)\right] &= \delta(x-x')\psi_{\mathbf{e}_\alpha}(x,t). \end{aligned} \tag{S6}$$

Each set of $N$ electron operators defines a topological class of the quantum Hall system, which can be parametrized by the $K$ matrix

$$K_{\alpha\beta} = \mathbf{e}_\alpha \cdot \mathbf{e}_\beta \tag{S7}$$

---

* kishore.iyer@cpt.univ-mrs.fr

Then all the allowed quasiparticle operators $\psi_{\mathbf{g}} \sim e^{i\mathbf{g}\cdot\boldsymbol{\phi}}$ are found by demanding that they commute or anti-commute with the electron operators

$$\psi_{\mathbf{g}}(x,t)\psi_{\mathbf{e}_\alpha}(x',t) \pm \psi_{\mathbf{g}}(x',t), \psi_{\mathbf{e}_\alpha}(x,t) = 0 \tag{S8}$$

For tunneling of quasiparticles at a QPC, within a low energy approximation, the quasiparticles with the lowest scaling dimension have the highest tunneling probability. Hence, the ones with higher scaling dimensions are usually ignored, as is done in this work. We emphasize that the parameters $N$, $\mathbf{q}$, and $\chi$ here are phenomenological, with the values chosen below being motivated by experimental observations.

Having calculated the quasiparticle operators in a given edge theory, their relevant properties are given as follows. The charge of $\psi_{\mathbf{g}}$ is given by

$$q_{\mathbf{g}} = \mathbf{g}.\mathbf{q}\ e \tag{S9}$$

the scaling dimension is given by

$$\delta_{\mathbf{g}} = \sum_i g_i^2 \tag{S10}$$

while the mutual exchange statistics of two different quasiparticle types $\psi_{\mathbf{g_1}}$ and $\psi_{\mathbf{g_2}}$ is given by

$$\theta_{\mathbf{g_1 g_2}} \equiv \pi\lambda_{\mathbf{g_1 g_2}} = \pi\ \mathbf{g_1}.\mathbf{g_2} \tag{S11}$$

## Laughlin states

Laughlin states are observed for the FQHE at filling factor $\nu = 1/(2m+1)$ (with $m$ and integer). The edge theory is described by a single Luttinger liquid ($N = 1$), with $\mathbf{q} = (\sqrt{\nu})$, and $\mathbf{g} = (\sqrt{\nu})$. This gives for the electron operator, $\mathbf{e} = (\mathbf{1}/\sqrt{\nu})$ and hence a trivial K-matrix, $(1/\nu)$. This recovers the usual results: the quasiparticle operator is given by $\psi_{\mathbf{g}} \sim e^{i\sqrt{\nu}\phi}$, quasiparticle charge is $q_{\mathbf{g}} = \nu e$, the exchange statistics is $\theta_{\mathbf{gg}} = \pi\nu$, and finally the scaling dimension is $\delta_{\mathbf{g}} = \nu$.

## $\boldsymbol{\nu = 2/5}$

Theoretically describing the $\nu = 2/5$ FQHE state requires two chiral Luttinger liquids on the edge ($N = 2$) which is consistent with experiments. Moreover, experiment results suggest the presence of two edge modes with conductance 1/3 and 1/15 respectively, giving us $\mathbf{q} = (\sqrt{1/3}, \sqrt{1/15})$. Both modes propagate in the same direction, hence $\chi = (+\mathbf{1}, +\mathbf{1})$. This choice of $\mathbf{q}$ and $\chi$ satisfies Eq. (S4) and gives us for the electron operators

$$\begin{aligned} \mathbf{e_1} &= \left(-2/\sqrt{3}, -\sqrt{5/3}\right) \\ \mathbf{e_2} &= \left(-\sqrt{3}, 0\right) \end{aligned} \tag{S12}$$

and hence the K-matrix

$$K = \begin{pmatrix} 3 & 2 \\ 2 & 3 \end{pmatrix} \tag{S13}$$

From these, it can then be shown that there exist two quasiparticles of the lowest scaling dimension, having charge $e/5$ [S3]. They are given by $e^{i\mathbf{g_1}\cdot\boldsymbol{\phi}}$ and $e^{i\mathbf{g_2}\cdot\boldsymbol{\phi}}$, where

$$\begin{aligned} \mathbf{g_1} &= \left(0, \sqrt{3/5}\right) \\ \mathbf{g_2} &= \left(\sqrt{1/3}, -2/\sqrt{15}\right) \end{aligned} \tag{S14}$$

Both of these charge $e/5$ quasiparticles have the same scaling dimension $\delta_{\mathbf{g_1}} = \delta_{\mathbf{g_2}} = 3/5$. Their exchange statistics is given by $\theta_{\mathbf{g_1 g_1}} = \theta_{\mathbf{g_2 g_2}} = \theta_{\mathbf{g_1 g_2}} = 3\pi/5$.

Since all the relevant quantities: charge, scaling dimension and exchange statistics are the same for both $\psi_{\mathbf{g_1}}$ and $\psi_{\mathbf{g_2}}$, the features of the multiple chiral Luttinger liquid model can be captured simply by using a single chiral Luttinger liquid model with $e^* = e/5$, $\delta = 3/5$, and $\theta = 3\pi/5$, as done in the main text. In general, such a simplification can always be carried out for all fully chiral quantum Hall edges [$\boldsymbol{\chi} = (+1, \ldots, +1)$].

## II. CURRENT DUE TO SINGLE QUASIPARTICLE: GENERAL ABELIAN QUANTUM HALL EDGE

In this section, we calculate the tunneling current due to a single quasiparticle incident on the quantum point contact, using the general theory recalled in the previous section. For simplicity, we make the assumption of a single type of quasiparticle tunneling across the QPC (generalization is straightforward). The tunneling Hamiltonian at the QPC is given by

$$H_T(t) = \Gamma\left(e^{i\mathbf{g_1}\cdot\boldsymbol{\phi}^{\mathbf{u}} - i\mathbf{g_1}\cdot\boldsymbol{\phi}^{\mathbf{d}}} + \text{H.c.}\right) \tag{S15}$$

while the tunneling current from the upper edge to the lower edge is

$$I_T(t) = iq_{\mathbf{g_1}}\Gamma\left(e^{i\mathbf{g_1}\cdot\boldsymbol{\phi}^{\mathbf{u}} - i\mathbf{g_1}\cdot\boldsymbol{\phi}^{\mathbf{d}}} - \text{H.c.}\right) \tag{S16}$$

A single quasiparticle flows on the upper edge, hitting the QPC at time $t_0$. This process is modelled by augmenting the bosonic field $\boldsymbol{\phi^u}$ with a solitonic excitation

$$\phi_i^u \longrightarrow \phi_i^u + 2\pi g_{2i}\left[\frac{1}{\pi}\tan^{-1}\left(\frac{t-t_0}{t_w}\right) + \frac{1}{2}\right] \tag{S17}$$

where we have assumed for the sake of illustration, that the quasiparticle tunneling across the QPC, and the one impinging on the QPC are of different types. The tunneling current in the QPC can be expressed, to leading order in the tunneling constant, within the Keldysh formalism as

$$\langle I_T(t)\rangle = -\frac{i}{2}\int dt' \sum_{\eta\eta'} \eta' \left\langle\left\{T_K\ I_T(t^\eta) H_T(t'^{\eta'})\right\}\right\rangle \tag{S18}$$

where $\eta, \eta'$ denote the Keldysh contour labels, and $T_K$ denotes time ordering on the Keldysh contour. We plug in the tunneling Hamiltonian and tunneling current operators

$$\langle I_T(t)\rangle = \frac{q_{\mathbf{g_1}}\Gamma^2}{2}\int dt' \sum_{\epsilon\eta\eta'} \epsilon\eta' \left\langle\left\{T_K\ \left[e^{i\mathbf{g_1}\cdot\boldsymbol{\phi}^u(t^\eta) - i\mathbf{g_1}\cdot\boldsymbol{\phi}^d(t^\eta)}\right]^{\epsilon}\left[e^{i\mathbf{g_1}\cdot\boldsymbol{\phi}^u(t'^{\eta'}) - i\mathbf{g_1}\cdot\boldsymbol{\phi}^d(t'^{\eta'})}\right]^{-\epsilon}\right\}\right\rangle \tag{S19}$$

where the sum over $\epsilon$ exists to account for both terms in Eqs. (S15) and (S16). We can further expand this as

$$\begin{aligned}\langle I_T(t)\rangle = \frac{q_{\mathbf{g_1}}\Gamma^2}{2}\int dt' \sum_{\epsilon\eta\eta'} \epsilon\eta' \prod_j \left\langle\left\{T_K\ e^{i\epsilon g_{1j}\phi_j^u(t^\eta)} e^{-i\epsilon g_{1j}\phi_j^u(t'^{\eta'})}\right\}\right\rangle \left\langle\left\{T_K\ e^{-i\epsilon g_{1j}\phi_j^d(t^\eta)} e^{i\epsilon g_{1j}\phi_j^d(t'^{\eta'})}\right\}\right\rangle \\ \times \exp\left\{2\epsilon g_{1j} g_{2j}\left[\tan^{-1}\left(\frac{t-t_0}{t_w}\right) - \tan^{-1}\left(\frac{t'-t_0}{t_w}\right)\right]\right\}\end{aligned} \tag{S20}$$

Using now the identity,

$$\left\langle\left\{T_K\ e^{i\epsilon g_{1j}\phi_j^{u/d}(t^\eta)} e^{-i\epsilon g_{1j}\phi_j^{u/d}(t'^{\eta'})}\right\}\right\rangle = e^{g_{1j}^2 \mathcal{G}_j^{\eta\eta'}(t-t')} \tag{S21}$$

where $\mathcal{G}^{\eta\eta'}(t)$ denotes the components of the Keldysh Green's function for the bosonic modes, and summing over $\epsilon$, we get

$$\langle I_T(t)\rangle = 2iq_{\mathbf{g_1}}\Gamma^2 \int dt' \sum_{\eta\eta'} \eta' \prod_j e^{2g_{1j}^2 \mathcal{G}_j^{\eta\eta'}(t-t')}\ \sin\left\{2\sum_j g_{1j} g_{2j}\left[\tan^{-1}\left(\frac{t-t_0}{t_w}\right) - \tan^{-1}\left(\frac{t'-t_0}{t_w}\right)\right]\right\} \tag{S22}$$

Summing now over the Keldysh contour indices and using the relations between different components of the Keldysh Green's function [S4], the current takes the form

$$\langle I_T(t)\rangle = 2iq_{\mathbf{g_1}}\Gamma^2 \int_{-\infty}^{t} dt' \left(e^{\sum_j 2g_{1j}^2 \mathcal{G}_j(t-t')} - e^{\sum_j 2g_{1j}^2 \mathcal{G}_j(t'-t)}\right) \sin\left\{2\sum_j g_{1j} g_{2j}\left[\tan^{-1}\left(\frac{t-t_0}{t_w}\right) - \tan^{-1}\left(\frac{t'-t_0}{t_w}\right)\right]\right\} \tag{S23}$$

where the summation inside the sine includes only the bosonic modes flowing towards the QPC, and

$$\mathcal{G}_j(t) \equiv \mathcal{G}_j^{-+}(t) = \ln\left(\frac{\sinh(i\pi k_B T\tau_{0j}/\hbar)}{\sinh[\pi k_B T(t-i\tau_{0j})/\hbar]}\right) \tag{S24}$$

where $\tau_{0j}$ is the cutoff corresponding to the $j-$th bosonic mode. We then have

$$\sum_j g_j^2 = \delta_{\mathbf{g}} \tag{S25}$$

and for fully chiral edges [S5],

$$\sum_j g_{1j}g_{2j} \equiv \mathbf{g_1}\cdot\mathbf{g_2} = \lambda_{\mathbf{g_1}\mathbf{g_2}} \equiv \theta_{g_1 g_2}/\pi \tag{S26}$$

representing the exchange phase of the quasiparticles $\psi_{\mathbf{g_1}}$ and $\psi_{\mathbf{g_2}}$. Finally, in the limit $\tau_{0j}\to 0$

$$\mathcal{G}_j(t) \equiv \mathcal{G}(t) = \ln\left(\frac{\sinh(i\pi k_B T\tau_0/\hbar)}{\sinh[\pi k_B T(t-i\tau_0)/\hbar]}\right) \tag{S27}$$

for all $j$, where $\tau_0$ is smaller than the smallest $\tau_{0j}$. With this, we can write for fully chiral edges

$$\langle I_T(t)\rangle = 2iq_{\mathbf{g_1}}\Gamma^2\int_{-\infty}^{t} dt'\left(e^{2\delta_{\mathbf{g_1}}\mathcal{G}(t-t')} - e^{2\delta_{\mathbf{g_1}}\mathcal{G}(t'-t)}\right)\sin\left\{2\lambda_{\mathbf{g_1}\mathbf{g_2}}\left[\tan^{-1}\left(\frac{t-t_0}{t_w}\right)-\tan^{-1}\left(\frac{t'-t_0}{t_w}\right)\right]\right\} \tag{S28}$$

From the above one can see that the current through the QPC for an edge theory with multiple bosonic modes can be simply captured using a single chiral Luttinger liquid expression, via the appropriate choice of the parameters $q_{\mathbf{g_1}}$, $\delta_{\mathbf{g_1}}$ and $\lambda_{\mathbf{g_1}\mathbf{g_2}}$, as done in the main text.

## III. THEORY OF THE ANYON COLLIDER

We outline here the theory of the anyon collider, following Ref. S6. The geometry of the anyon collider comprises three QPCs. The QPCs on the left and right are biased with a voltage $V$, and are placed in the weak-backscattering regime. These QPCs emit fractional quasiparticles on the opposite edges, which then travel downstream toward the central QPC. The left and right QPCs, called source QPCs henceforth, act as sources of random streams of quasiparticles for the central QPC. The stream of incoming quasiparticles can be modeled by augmenting the bosonic fields with solitons as

$$\phi_i^{u/d} \longrightarrow \phi_i^{u/d} + 2\pi g_i\sum_k\left[\frac{1}{\pi}\tan^{-1}\left(\frac{t-t_k^{u/d}}{t_w}\right)+\frac{1}{2}\right] \tag{S29}$$

where the times $t_k^{u/d}$ denote the time at which the $k$-th quasiparticle on the upper/lower edge hits the central QPC, and these times follow a Poissonian distribution. We have assumed here that a single type of quasiparticle is emitted on the edges from the source QPCs. The Poissonian stream of quasiparticles gives rise to an average input current $I_{u/d}$ on the upper/lower edge. The average tunneling current at the central QPC can be expressed with the Keldysh formalism as

$$\langle I_T\rangle = -\frac{i}{2}\int dt'\sum_{\eta\eta'}\eta'\left\langle\left\{T_K\ I_T(t^\eta)H_T(t'^{\eta'})\right\}\right\rangle \tag{S30}$$

where $\eta,\eta'$ denote the Keldysh contour labels, and $T_K$ denotes time ordering on the Keldysh contour. The tunneling Hamiltonian $H_T(t)$ is given by

$$H_T(t) = \Gamma\left(e^{i\mathbf{g}\cdot\boldsymbol{\phi}_{\mathbf{u}}}e^{-i\mathbf{g}\cdot\boldsymbol{\phi}_{\mathbf{d}}}+\text{H.c.}\right) \tag{S31}$$

where we have assumed that a single type of quasiparticle tunnels across the central QPC. The tunneling current can then be shown to take the form [S4, S6, S7]

$$\langle I_T\rangle = 2ie^*\Gamma^2\int_0^\infty dt\quad\frac{\sin\left[x\text{Im}f(t,\lambda,\tau_w)\right]}{\exp\left[\text{Re}f(t,\lambda,\tau_w)\right]}\left(e^{2\delta\mathcal{G}(t)}-e^{2\delta\mathcal{G}(-t)}\right) \tag{S32}$$

where $x = I_+/I_-$, $I_\pm = I_u \pm I_d$, and the phase accumulated due to the finite width of quasiparticles is given by

$$f(t,\lambda,\tau_w) = \int_{-\infty}^{\infty} du \left\{ 1 - \exp\Big( -2i\lambda\Big[ \tan^{-1}\left(\frac{t/t_s - u}{\tau_w}\right) - \tan^{-1}\left(\frac{0-u}{\tau_w}\right)\Big]\Big)\right\} \tag{S33}$$

The tunneling noise at the QPC can be expressed as

$$\langle S_T \rangle = \int dt' \sum_\eta \langle \{ T_K \; I_T(t^\eta) I_T(t'^{-\eta}) \} \rangle \tag{S34}$$

which after some manipulations gives us [S4, S6, S7]

$$\langle S_T \rangle = e^{2*}\Gamma^2 \int_0^\infty dt \; \frac{\cos\left[x \mathrm{Im} f(t,\lambda,\tau_w)\right]}{\exp\left[\mathrm{Re} f(t,\lambda,\tau_w)\right]} \left( e^{2\delta\mathcal{G}(t)} + e^{2\delta\mathcal{G}(-t)} \right) \tag{S35}$$

In the limit $t_w \longrightarrow 0$, these assume the form quoted in Ref. S6

$$\langle I_T \rangle = 2ie^*\Gamma^2 \int_0^\infty dt \; \frac{\sin\left[\frac{I_-}{e^*} t \sin(2\pi\lambda)\right]}{\exp\left[\frac{I_+}{e^*} t(1-\cos(2\pi\lambda))\right]} \left( e^{2\delta\mathcal{G}(t)} - e^{2\delta\mathcal{G}(-t)} \right) \tag{S36}$$

$$\langle S_T \rangle = e^{2*}\Gamma^2 \int_0^\infty dt \; \frac{\cos\left[\frac{I_-}{e^*} t \sin(2\pi\lambda)\right]}{\exp\left[\frac{I_+}{e^*} t(1-\cos(2\pi\lambda))\right]} \left( e^{2\delta\mathcal{G}(t)} + e^{2\delta\mathcal{G}(-t)} \right) \tag{S37}$$

The current cross-correlations, which are accessible experimentally, are related to the tunneling noise and tunneling current via a fluctuation-dissipation relation

$$\langle \delta I_u \delta I_d \rangle = -\langle S_T \rangle + e^* \left( I_+ \tfrac{\partial}{\partial I_-} + I_- \tfrac{\partial}{\partial I_+} \right) \langle I_T \rangle \tag{S38}$$

Finally, we define a generalized Fano factor, dividing the cross-correlations by the differential transmission of the QPC

$$P(x = I_-/I_+) = \frac{\langle \delta I_u \delta I_d \rangle}{e^* I_+ \frac{\partial \langle I_T \rangle}{\partial I_-}\Big|_{I_-=0}} \tag{S39}$$

## IV. FINITE WIDTH QUASIPARTICLES WITH A RECTANGULAR PROFILE

In the main text, we considered finite width quasiparticles with a Lorentzian profile (see e.g. Eq.(1) of the main text, where the $\tan^{-1}$ correspond the integration of a Lorentzian), and showed how the finite width impacts physical quantities measured at a QPC. We consider here a different profile for finite-width quasiparticles, and show that the results are qualitatively the same. We chose here to use a rectangular profile, as it corresponds to the case of a maximally sharp profile (qp density exactly 0 outside the rectangular width), while the lorentzian profile used in the main text corresponds to a quasiparticle with a long tail (qp density decreasing $\sim 1/x^2$). Other profiles of quasiparticles should give results which are intermediate between these two cases. For the case of the rectangular profile, the tunneling current and noise can be shown to be

$$\begin{aligned} \langle I_T \rangle &= 2ie^*\Gamma^2 \int_0^\infty dt \; \frac{\sin\left[x \mathrm{Im} g(t,\lambda,\tau_w)\right]}{\exp\left[\mathrm{Re} g(t,\lambda,\tau_w)\right]} \left( e^{2\delta\mathcal{G}(t)} - e^{2\delta\mathcal{G}(-t)} \right) \\ \langle S_T \rangle &= e^{2*}\Gamma^2 \int_0^\infty dt \; \frac{\cos\left[x \mathrm{Im} g(t,\lambda,\tau_w)\right]}{\exp\left[\mathrm{Re} g(t,\lambda,\tau_w)\right]} \left( e^{2\delta\mathcal{G}(t)} + e^{2\delta\mathcal{G}(-t)} \right) \end{aligned} \tag{S40}$$

with the only difference with the Lorentzian profile case (Eq. (6) of the main text, and Eq.(S35) of the SM) being in the phase function $g(t,\lambda,t_w)$, the phase gathered at the QPC due to rectangular finite-width quasiparticles. This can be expressed as

$$g(t,\lambda,t_w) = \int_{-\infty}^{\infty} \left[ 1 - \exp\left\{ -\frac{2i\pi\lambda}{t_w} \left( \left[ (t_w+u) - (t_w+u)\Theta(-t_w-u) - t \right] \Theta(t-t_w-u) - \left[ u - u\Theta(-u) - t \right] \Theta(t-u) \right) \right\} \right] \tag{S41}$$

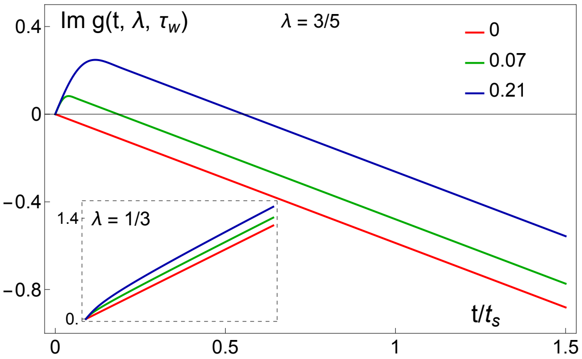


FIG. S1. Imaginary part of the finite-width phase due to rectangular quasiparticles as a function of time for $\lambda = 3/5$, for scaled width $\tau_w = 0, 0.07, 0.21$. Qualitatively, the behaviour is similar to Lorentzian quasiparticles presented in Fig.2 of the main text where the slope is equal to $\sin(2\pi * 3/5)(t/t_s)$ for $\tau_w = 0$, but becomes positive at small time $t$ for non zero $\tau_w$. In contrast with Lorentzian quasiparticles, the change of slope from positive to negative is more abrupt for rectangular quasiparticles. As a consequence, a same scaled width $t_w$ will have a smaller quantitative effect for rectangular quasiparticles compared to Lorentzian ones. Inset: same curves for $\lambda = 1/3$, showing that for $\lambda < 1/2$ a finite width does not significantly change the phase.

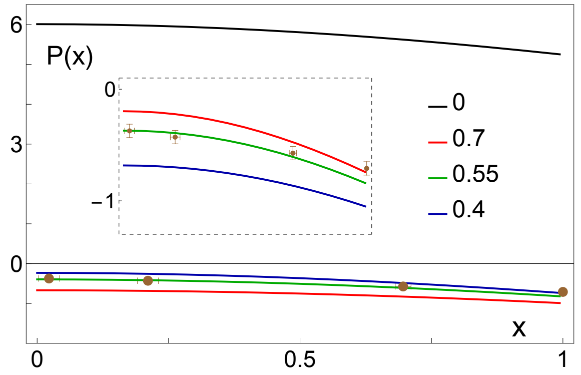


FIG. S2. Generalized Fano factor of Eq. (S39) plotted as a function of the current asymmetry for rectangular quasiparticles hitting the QPC (compare with Fig.3b of the main text). We achieve a reasonable agreement with experimental data for $\tau_w = 0.55$, a factor $\sim 7$ larger than the value $\tau_w = 0.075$ found for Lorentzian quasiparticles.

where $\Theta(x)$ is the Heaviside step function. Again, the limit $t_w \longrightarrow 0$ recovers the results of Ref. [S6].

We consider first the phase function $g(t, \lambda, t_w)$ for different values of the width $t_w$ in Figure S1 (to be compared with Fig. 2 of the main text), for $\lambda = 1/3$ and $\lambda = 3/5$. For $\lambda = 1/3$, $t_w = 0$ implies a positive slope of Im$g(t, \lambda, t_w)$, and increasing the width quantitatively changes the slope, but does not lead to drastic changes. In contrast, at $\lambda = 3/5$, Im$g(t, \lambda, t_w)$ displays a negative slope for $t_w = 0$. When $t_w$ is non-zero, the slope becomes positive close to $t = 0$, and eventually recovers a negative slope. The behavior of the phase for rectangular quasiparticles is qualitatively the same as that for Lorentzian quasiparticles, presented in the Fig.2 of the main text. But in contrast with Lorentzian quasiparticles, the change in slope from positive to negative for large $t$ in Fig. S1 is more abrupt in the case of rectangular quasiparticles. This is a consequence of the profile of the quasiparticles: Lorentzian quasiparticles have a long tail and vary smoothly, leading to a smooth change in the effective phase seen at the QPC. On the other hand, rectangular quasiparticles have no tails and vary abruptly, leading to the behaviour seen in Fig. S1. To achieve quantitative agreement between Lorentzian and rectangular quasiparticles, we find that a larger finite width is needed for rectangular quasiparticles. Fig. S2 (to be ocmpared with Fig.3b of the main text) shows the behavior of the P-value measured in experiments for different values of finite width of the rectangular quasiparticles. Agreement with experiments is achieved at $\tau_w = 0.55$, a factor of $\sim 7$ larger than the $\tau_w$ needed for Lorentzian quasiparticles.

Since different shapes of quasiparticles leads to agreement with experiments for different scaled widths, a comprehensive study of the effect of shapes of quasiparticles on the transport properties is required. Here, we illustratively consider two extreme limits of shapes: Lorentzian quasiparticles having long tails, and rectangular quasiparticles having no tails. Both achieve an order-of-magnitude agreement with experimentally used values of QPC transparency.

## V. CONNECTION BETWEEN THE SIGN OF CURRENT AND THE BRAIDING PHASE

In this section, we interpret the change of sign in the current in terms of the braiding phase of the anyons. For simplicity, we will focus on the case where only one type of quasi-particle exists with its corresponding quasi-hole. In this sense the mutual statistical exchange is given by

$$\lambda_{pp} = \lambda_{hh} = 1 - \lambda_{ph} = 1 - \lambda_{hp} \equiv \lambda \tag{S42}$$

where $p$ corresponds to the quasi-particle and $h$ to the quasi-hole and the choice of writing $1 - \lambda_{ph}$ and $1 - \lambda_{hp}$ is due to the fact that we want to ensure $0 < \lambda < 1$. Eq.(S42) means that the double exchange phase between two quasiparticles is given by $\exp(2i\pi\lambda_{pp})$. For instance, in the case of $\nu = 1/3$, one has $\lambda = 1/3$, which implies $\lambda_{pp} = 1/3$ and $\lambda_{ph} = 2/3$. Despite the $\lambda = 1/2$ case being unphysical, it is instructive to notice that in this case $\lambda_{pp} = \lambda_{ph}$. In this sense the case $\lambda = 1/2$ is special and denotes a symmetric point. Indeed, one can observe that if $\lambda_{pp} < 1/2$ ($\lambda_{pp} > 1/2$), then one has $\lambda_{ph} > 1/2$ ($\lambda_{ph} < 1/2$). Due to this symmetry, the role of quasi-particles and quasi-holes is exchanged between theories with $0 < \lambda < 1/2$ and theories with $1/2 < \lambda < 1$.

For illustration, we consider a single anyonic excitation incoming on a QPC, and compute the tunneling current. Here, we focus on the case of zero-width excitations, since the relation between $\lambda$ and the sign of the current does not require to take into account the finite width. The effect of the latter is to reduce the effective value of $\lambda$. All the technical details for the calculation of the tunneling current can be found in Ref.[S8]. It is useful to recast the current as

$$I^{(\lambda)} = \left(\Gamma_+^{(\lambda)}(t) - \Gamma_-^{(\lambda)}(t)\right) e^* \tag{S43}$$

where we introduce the tunneling rates

$$\Gamma_+^{(\lambda)}(t) = |\Gamma|^2 \int_{-\infty}^{t} dt' \ \left[\left\langle \varphi \left| \psi_R^\dagger(t)\psi_R(t') \right| \varphi \right\rangle \left\langle 0 \left| \psi_L(t)\psi_L^\dagger(t') \right| 0 \right\rangle + \left\langle \varphi \left| \psi_R^\dagger(t')\psi_R(t) \right| \varphi \right\rangle \left\langle 0 \left| \psi_L(t')\psi_L^\dagger(t) \right| 0 \right\rangle\right] \tag{S44}$$

$$= |\Gamma|^2 \int_{-\infty}^{t} dt' \ \left[\left\langle \varphi \left| \psi_R^\dagger(t)\psi_R(t') \right| \varphi \right\rangle e^{2\delta\mathcal{G}(t-t')} + \left\langle \varphi \left| \psi_R^\dagger(t')\psi_R(t) \right| \varphi \right\rangle e^{2\delta\mathcal{G}(t'-t)}\right], \tag{S45}$$

$$\Gamma_-^{(\lambda)}(t) = |\Gamma|^2 \int_{-\infty}^{t} dt' \ \left[\left\langle \varphi \left| \psi_R(t)\psi_R^\dagger(t') \right| \varphi \right\rangle \left\langle 0 \left| \psi_L^\dagger(t)\psi_L(t') \right| 0 \right\rangle + \left\langle \varphi \left| \psi_R(t')\psi_R^\dagger(t) \right| \varphi \right\rangle \left\langle 0 \left| \psi_L^\dagger(t')\psi_L(t) \right| 0 \right\rangle\right] \tag{S46}$$

$$= |\Gamma|^2 \int_{-\infty}^{t} dt' \ \left[\left\langle \varphi \left| \psi_R(t)\psi_R^\dagger(t') \right| \varphi \right\rangle e^{2\delta\mathcal{G}(t-t')} + \left\langle \varphi \left| \psi_R(t')\psi_R^\dagger(t) \right| \varphi \right\rangle e^{2\delta\mathcal{G}(t'-t)}\right], \tag{S47}$$

where $\psi_{R/L}$ are anyonic quasiparticle operators as defined in Eqn. S5, and $|\varphi\rangle$ is the state of the system with an incoming anyonic excitation on the edge $R$. Now we start discussing the physical meaning of these rates by focusing on the averages $\gamma_+ = \left\langle \varphi \left| \psi_R^\dagger(t)\psi_R(t') \right| \varphi \right\rangle$ and $\gamma_- = \left\langle \varphi \left| \psi_R(t)\psi_R^\dagger(t') \right| \varphi \right\rangle$, which carry all the information about braiding processes. Let us focus on $\gamma_+$ and make the average explicit. For a zero-width incoming excitation one has $|\varphi\rangle = \psi_R^\dagger(0)\,|0\rangle$ where the origin of time is chosen as the arrival time of the incoming quasi-particle at the QPC. This gives us the rate $\gamma_+$ to be

$$\gamma_+ = \left\langle \varphi \left| \psi_R^\dagger(t)\psi_R(t') \right| \varphi \right\rangle = \left\langle 0 \left| \psi_R(0)\psi_R^\dagger(t)\psi_R(t')\psi_R^\dagger(0) \right| 0 \right\rangle, \tag{S48}$$

Physically this term corresponds to the interference between different braiding processes. Because of the integrals in the tunneling rates we always have $t > t'$. If $t > 0$ and $t' < 0$ (resp. $t < 0$ and $t' < 0$) a quasi-particle/quasi-hole pair is created at the QPC after (resp. before) the injected quasi-particles passes through the QPC. In this sense the term $\gamma_+$ is the interference between the process where the injected quasi-particles ($\psi_R^\dagger(0)$) meets a quasi-hole from the QPC at time $t'$ ($\psi_R(t')$) and the process where the quasi-particle ($\psi_R(0)$) meets a quasi-hole from the QPC at time $t$ ($\psi_R^\dagger(t)$). We assume $t > 0$ and $t' < 0$, and then have

$$\gamma_+ = \left\langle 0 \left| \psi_R(0)\psi_R^\dagger(t)\psi_R(t')\psi_R^\dagger(0) \right| 0 \right\rangle = e^{i2\pi(1-\lambda)} \left\langle 0 \left| \psi_R^\dagger(t)\psi_R(0)\psi_R^\dagger(0)\psi_R(t') \right| 0 \right\rangle \tag{S49}$$

$$= e^{i2\pi\lambda_{ph}} \left\langle 0 \left| \psi_R^\dagger(t)\psi_R(0)\psi_R^\dagger(0)\psi_R(t') \right| 0 \right\rangle = e^{i2\pi\lambda_{ph}} e^{2\delta\mathcal{G}(t-t')}, \tag{S50}$$

where the phase $e^{2i\pi\lambda_{ph}}$ comes from the exchange between the $\psi_R(0)$ and $\psi_R^\dagger(t)$, and between $\psi_R^\dagger(0)$ and $\psi_R(t')$, and where we used $\psi_R(0)\psi_R^\dagger(0) = 1$ to recover the Green's function in the last equality. Let us move to $\gamma_-$ and make the

average explicit

$$\gamma_- = \left\langle \varphi \left| \psi_R(t)\psi_R^\dagger(t') \right| \varphi \right\rangle = \left\langle 0 \left| \psi_R(0)\psi_R(t)\psi_R^\dagger(t')\psi_R^\dagger(0) \right| 0 \right\rangle . \tag{S51}$$

In this case the injected quasi-particle is meeting the quasi-particle excited at the QPC and braids with it or not (depending on the values of $t$ and $t'$). As a result, for $t > 0$ and $t' < 0$, one has similarly to $\gamma_+$,

$$\gamma_- = \left\langle 0 \left| \psi_R(0)\psi_R(t)\psi_R^\dagger(t')\psi_R^\dagger(0) \right| 0 \right\rangle = e^{i2\pi\lambda} \left\langle 0 \left| \psi_R(t)\psi_R(0)\psi_R^\dagger(0)\psi_R^\dagger(t') \right| 0 \right\rangle \tag{S52}$$

$$= e^{i2\pi\lambda_{pp}} \left\langle 0 \left| \psi_R(t)\psi_R(0)\psi_R^\dagger(0)\psi_R^\dagger(t') \right| 0 \right\rangle = e^{i2\pi\lambda_{pp}} e^{2\delta\mathcal{G}(t-t')}. \tag{S53}$$

Therefore, one has

$$\Gamma_+^{(\lambda)}(t) = \Gamma_-^{(1-\lambda)}(t), \tag{S54}$$

which physically means that the difference between systems with $\lambda < 1/2$ and $\lambda > 1/2$ is that the braiding of the incoming quasi-particles with the quasi-particle (quasi-hole) is replaced by the braiding of the incoming quasi-particles with the quasi-hole (quasi-particle). In other words, the roles of quasi-particles and quasi-holes are exchanged in terms of statistics.

As a result, one also has that

$$I^{(\lambda)}(t) = -I^{(1-\lambda)}(t) \tag{S55}$$

and that, for delta-like particles,

$$\text{sign}\left[I^{(\lambda)}(t)\right] = \text{sign}\left(1/2 - \lambda\right) \tag{S56}$$

Since, for $\nu = 1/3$ one has $\lambda = 1/3 < 1/2$ and for $\nu = 2/5$ one has $\lambda = 3/5 > 1/2$, the sign of charge current in these two cases is opposite.


[S1] X.-G. Wen, Advances in Physics **44**, 405 (1995), https://doi.org/10.1080/00018739500101566.

[S2] O. Shtanko, K. Snizhko, and V. Cheianov, Phys. Rev. B **89**, 125104 (2014).

[S3] There exists a quasiparticle of charge 2e/5 that has an even lower scaling dimension, which we ignore as it is not seen in experiments.

[S4] T. Martin, in *Nanophysics: Coherence and Transport*, Les Houches, Session LXXXI, edited by H. Bouchiat, Y. Gefen, S. Guéron, G. Montambaux, and J. Dalibard (Elsevier, 2005) p. 283.

[S5] For non-chiral quantum Hall edges, such as $\nu = 2/3$, the phase inside the sine represents a partial exchange phase: of those parts of the quasiparticle flowing towards the QPC, with the corresponding parts tunneling at the QPC.

[S6] B. Rosenow, I. P. Levkivskyi, and B. I. Halperin, Phys. Rev. Lett. **116**, 156802 (2016).

[S7] N. Schiller, Y. Shapira, A. Stern, and Y. Oreg, Phys. Rev. Lett. **131**, 186601 (2023).

[S8] T. Jonckheere, J. Rech, B. Grémaud, and T. Martin, Phys. Rev. Lett. **130**, 186203 (2023).
